# Supplementary material for: Laplace Functional Ordering of Point Processes in Large-scale Wireless Networks
Source: arXiv:1408.4528 source file (2018-06-26)
Supplement: Supplementary file 6 [file appendix_Proof_for_min_max_Lf_pert_lat_PPs.tex]

\label{app:Proof_for_min_max_Lf_pert_lat_PPs}
The derivation follows \cite{Shaked}. The right side inequality in \eqref{eqn:Lt_ordering_of_RVs} follows from Jensen's inequality. Let $\overline{F}$ and $\overline{G}$ be the complementary cumulative distribution functions of $X$ and $Y$ respectively. In order to obtain the left side inequality in \eqref{eqn:Lt_ordering_of_RVs} we will show that
\begin{equation}
\int_{0}^{\infty} e^{-sx}\overline{F}(x)\mathrm{d}x \leq \int_{0}^{\infty} e^{-sx}\overline{G}(x)\mathrm{d}x \text{ for all } s \geq 0 \text{.}
\end{equation}  
The result will then follow from \cite[Theorem 5.A.1]{Shaked}.

Define the functions $\alpha$ and $\beta$ on $(0,\infty$ by $\alpha=\overline{F}(x)$ and $\beta=\overline{G}(x)$. In fact, $\alpha$ is the density function of the uniform distribution over the interval $[0,2)$, whereas $\beta$ is a density which is decreasing on $[0,\infty)$. From \cite[Theorem 3.A.46]{Shaked} it now follows that
\begin{equation}
\int_{0}^{\infty} \phi(x)\overline{F}(x)\mathrm{d}x \leq \int_{0}^{\infty} \phi(x)\overline{G}(x)\mathrm{d}x
\end{equation}
for all convex functions $\phi$, and $e^{-sx}$ is the convex function.
